# Supplementary material for: I Don't Miss You, but I Do: Self-Explanation Faithfulness of Modality Missingness in Vision-Language Models
Source: arXiv:2609.07596 source file (2026-09-30)
Supplement: Supplementary file 1 [file standalone_appendix.tex]

% Preview wrapper only - NOT part of the paper. It exists so appendix.tex can
% be compiled and eyeballed on its own:  latexmk -pdf paper/standalone.tex
\documentclass[11pt]{article}
\usepackage[margin=1in]{geometry}
\usepackage[T1]{fontenc}
\usepackage{natbib}

% The two lines to add to your own preamble:
\usepackage{booktabs,xcolor,listings,graphicx}
\usepackage[most]{tcolorbox}

\begin{document}
% \appendix
\input{appendix}
\bibliographystyle{plainnat}
\bibliography{refs}
\end{document}
